# Supplementary material for: VASSL: A Visual Analytics Toolkit for Social Spambot Labeling
Source: arXiv:1907.13319 source file (2019-10-07)
Supplement: Supplementary file 1 [file supplementalMaterials.tex]

\section{System Architecture}
Our system is built as a web-based application with front-end and back-end architecture. The front-end is written using HTML, CSS, and javascript. The interactive visualization is developed using both Vega \cite{2016-reactive-vega-architecture} and Vega-lite \cite{2017-vega-lite}. The design of VASSL requires a lot of interactions among views that are embedded in different sections of the HTML file, a requirement that can be achieved using Vega's dynamic variables known as signals.

The back-end of our system was built as a Node.js application that utilizes a set of modules including MySQL connector that connect our back-end to MySQL server that is running on the same machine. The back-end also spawns multiple child processes that run Python scripts to perform data preprocessing and automatic analysis. We use many libraries for these purposes including sci-kit-learn \cite{scikit-learn} for dimensionality reduction, NLTK \cite{bird2009natural} and Gensim \cite{rehurek_lrec} for natural language processing and topic modeling, Textblob \cite{loria2018textblob} for sentiment analysis.

The communication between the front-end and the back-end is facilitated by Socket.IO which enables async communication between the server and connected clients. Such a communication protocol allows clients to query the server on demand without the need to reload the page. The overall architecture of VASSL can be seen in figure \ref{fig:architecture}.

\begin{figure}[t]
 \centering 
 \includegraphics[width=\columnwidth]{architecture}
 \caption{The architecture of VASSL and the implementation environments.}
 \label{fig:architecture}
\end{figure}
